# Supplementary material for: BudgetFusion: Perceptually-Guided Adaptive Diffusion Models
Source: arXiv:2412.05780 source file (2024-12-23)
Supplement: Supplementary file 1 [file supplement.tex]

\appendixpageoff
\appendixtitleoff

\begin{appendices}
\crefalias{section}{supp}
\normalsize

% 
% \include{\jobname-support}

\end{appendices}

% \clearpage
% \appendixpageoff
% \appendixtitleoff
% \renewcommand{\appendixtocname}{Supplementary material}
% \begin{appendices}
% \crefalias{section}{supp}
% \normalsize

% 
% \include{\jobname-support}
% \end{appendices}
