# Supplementary material for: BudgetFusion: Perceptually-Guided Adaptive Diffusion Models
Source: arXiv:2412.05780 source file (2024-12-23)
Supplement: Supplementary file 3 [file tile_17.tex]

\begin{figure}
  \centering
  \includegraphics[width=\linewidth]{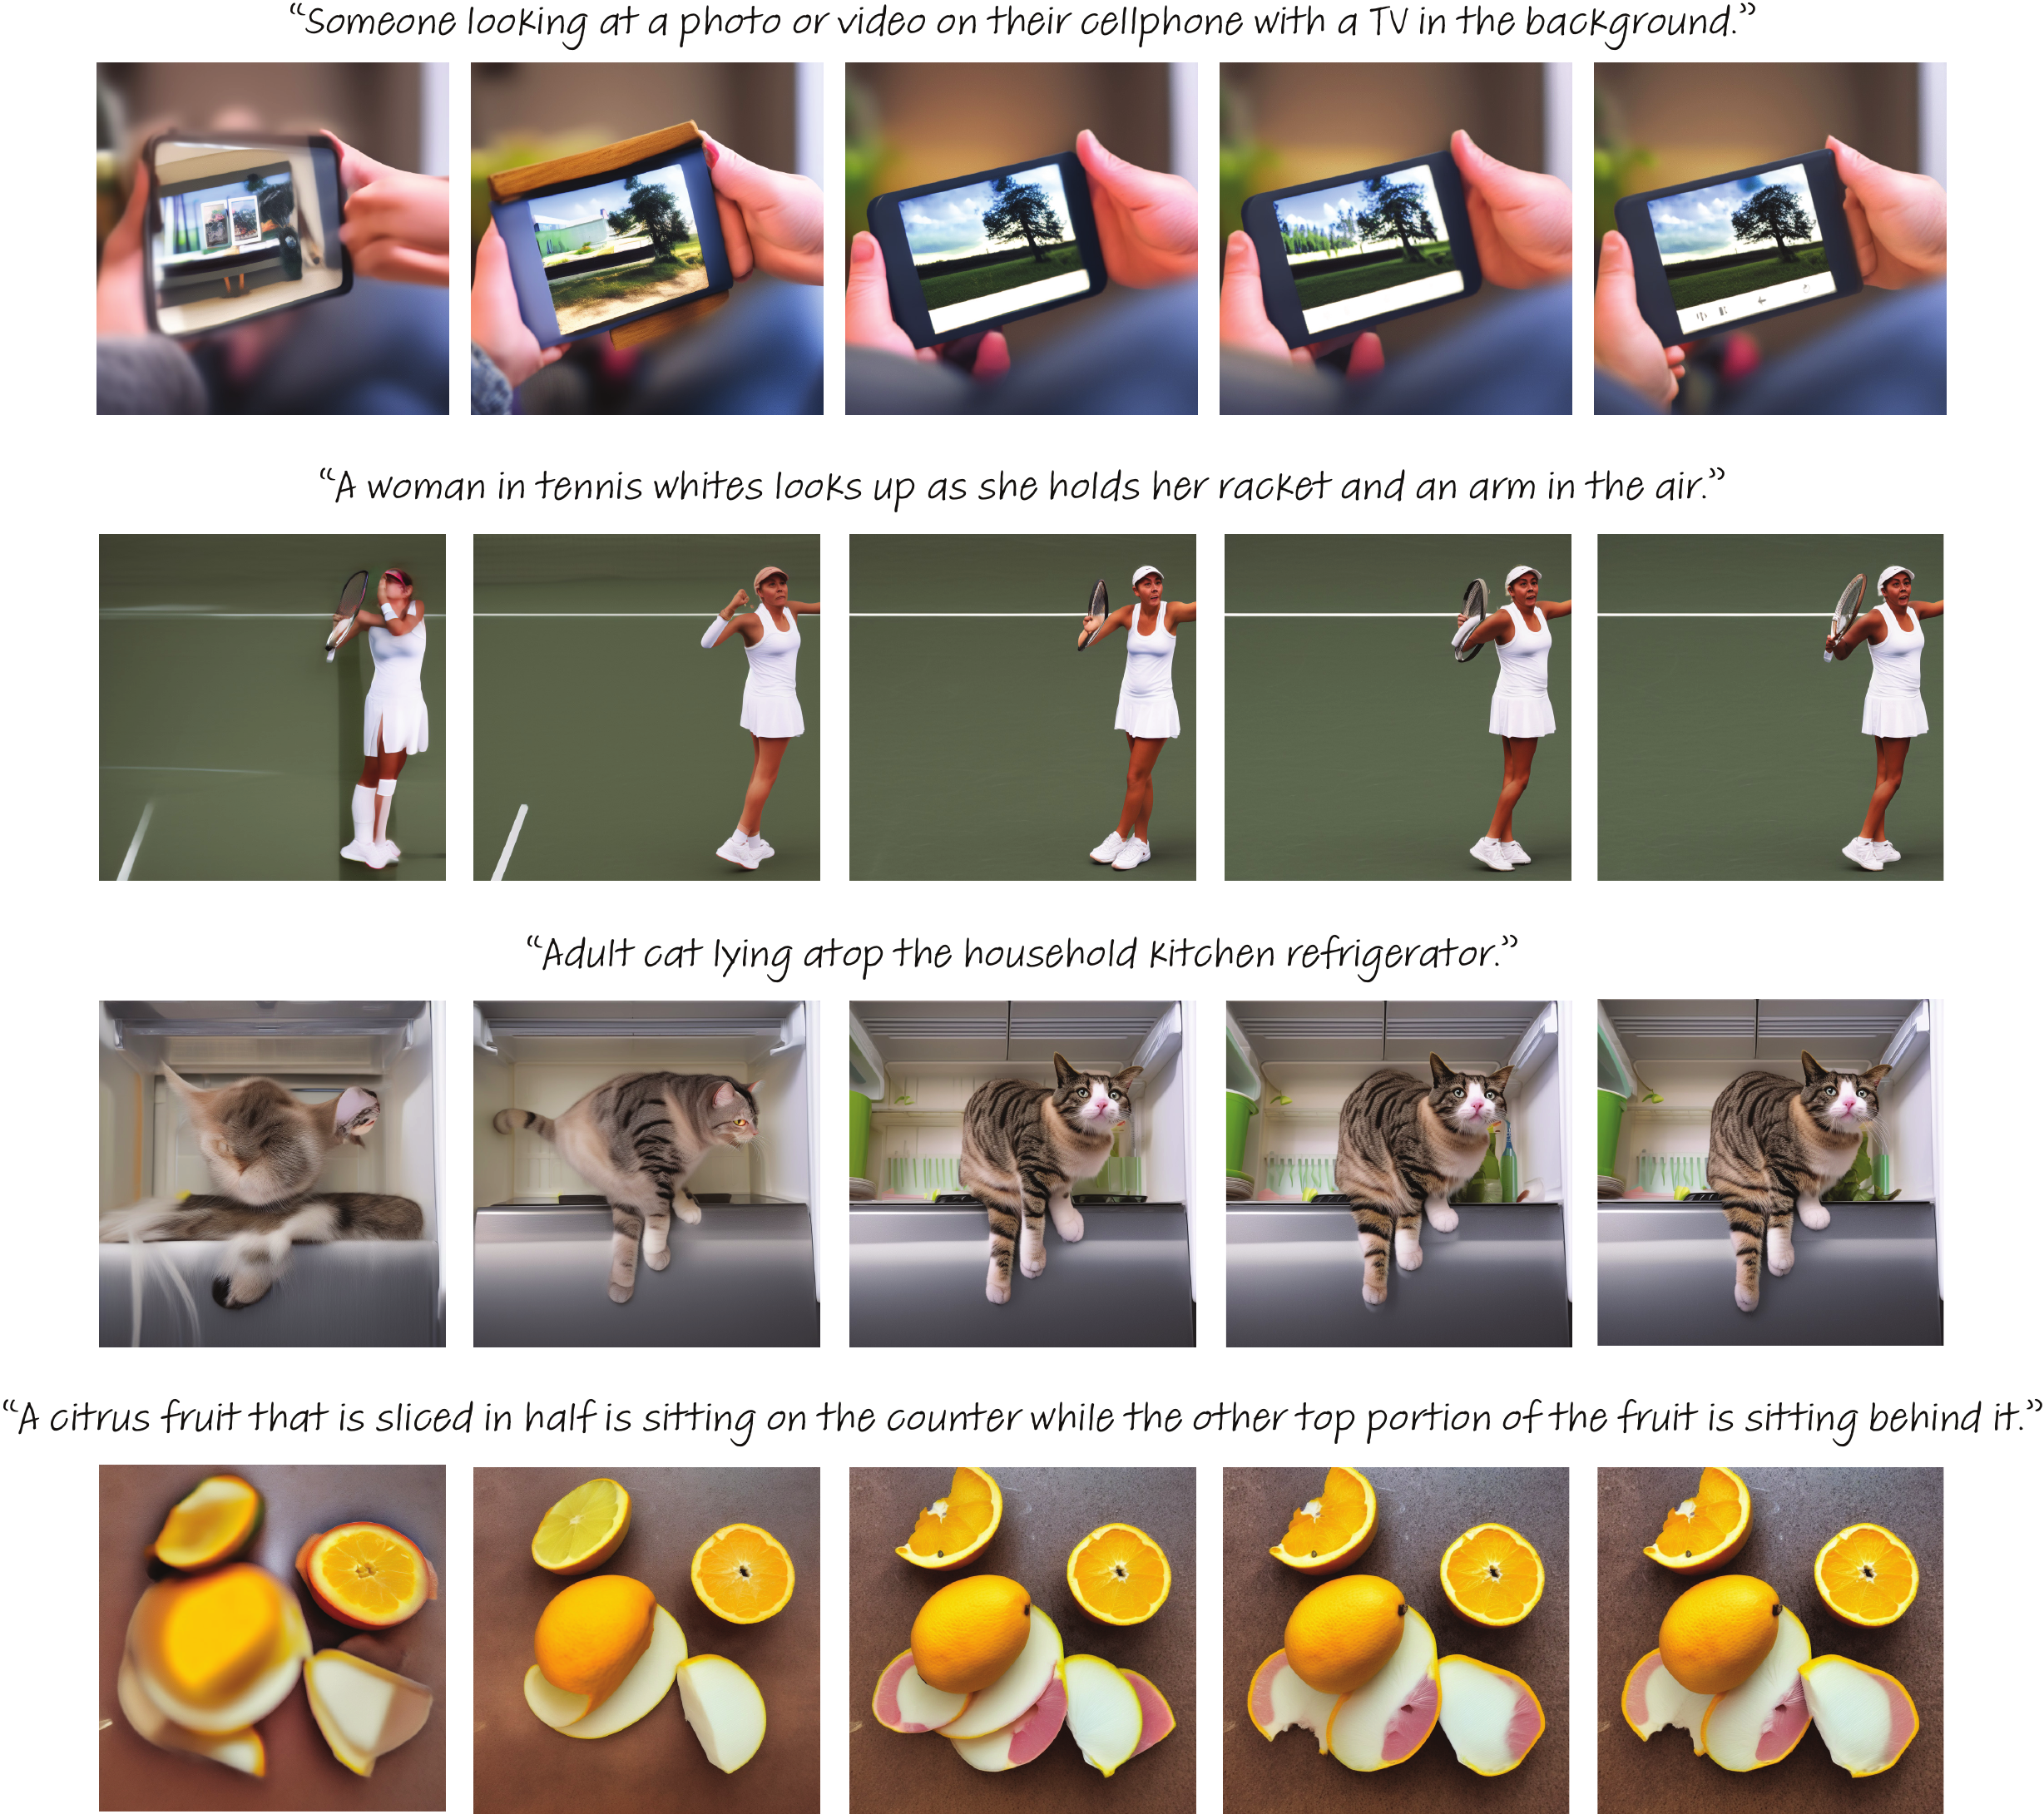}
  \Caption{
      Additional qualitative results at $t^*=17$.
  }{
    From left to right, the columns are $t=5,9,17,22,27$.
  }
  \label{fig:tileResults_17}
  \Description{}
\end{figure}
