# Supplementary material for: BudgetFusion: Perceptually-Guided Adaptive Diffusion Models
Source: arXiv:2412.05780 source file (2024-12-23)
Supplement: Supplementary file 4 [file tile_9.tex]

\begin{figure*}[h]
  \centering
  \includegraphics[width=\linewidth]{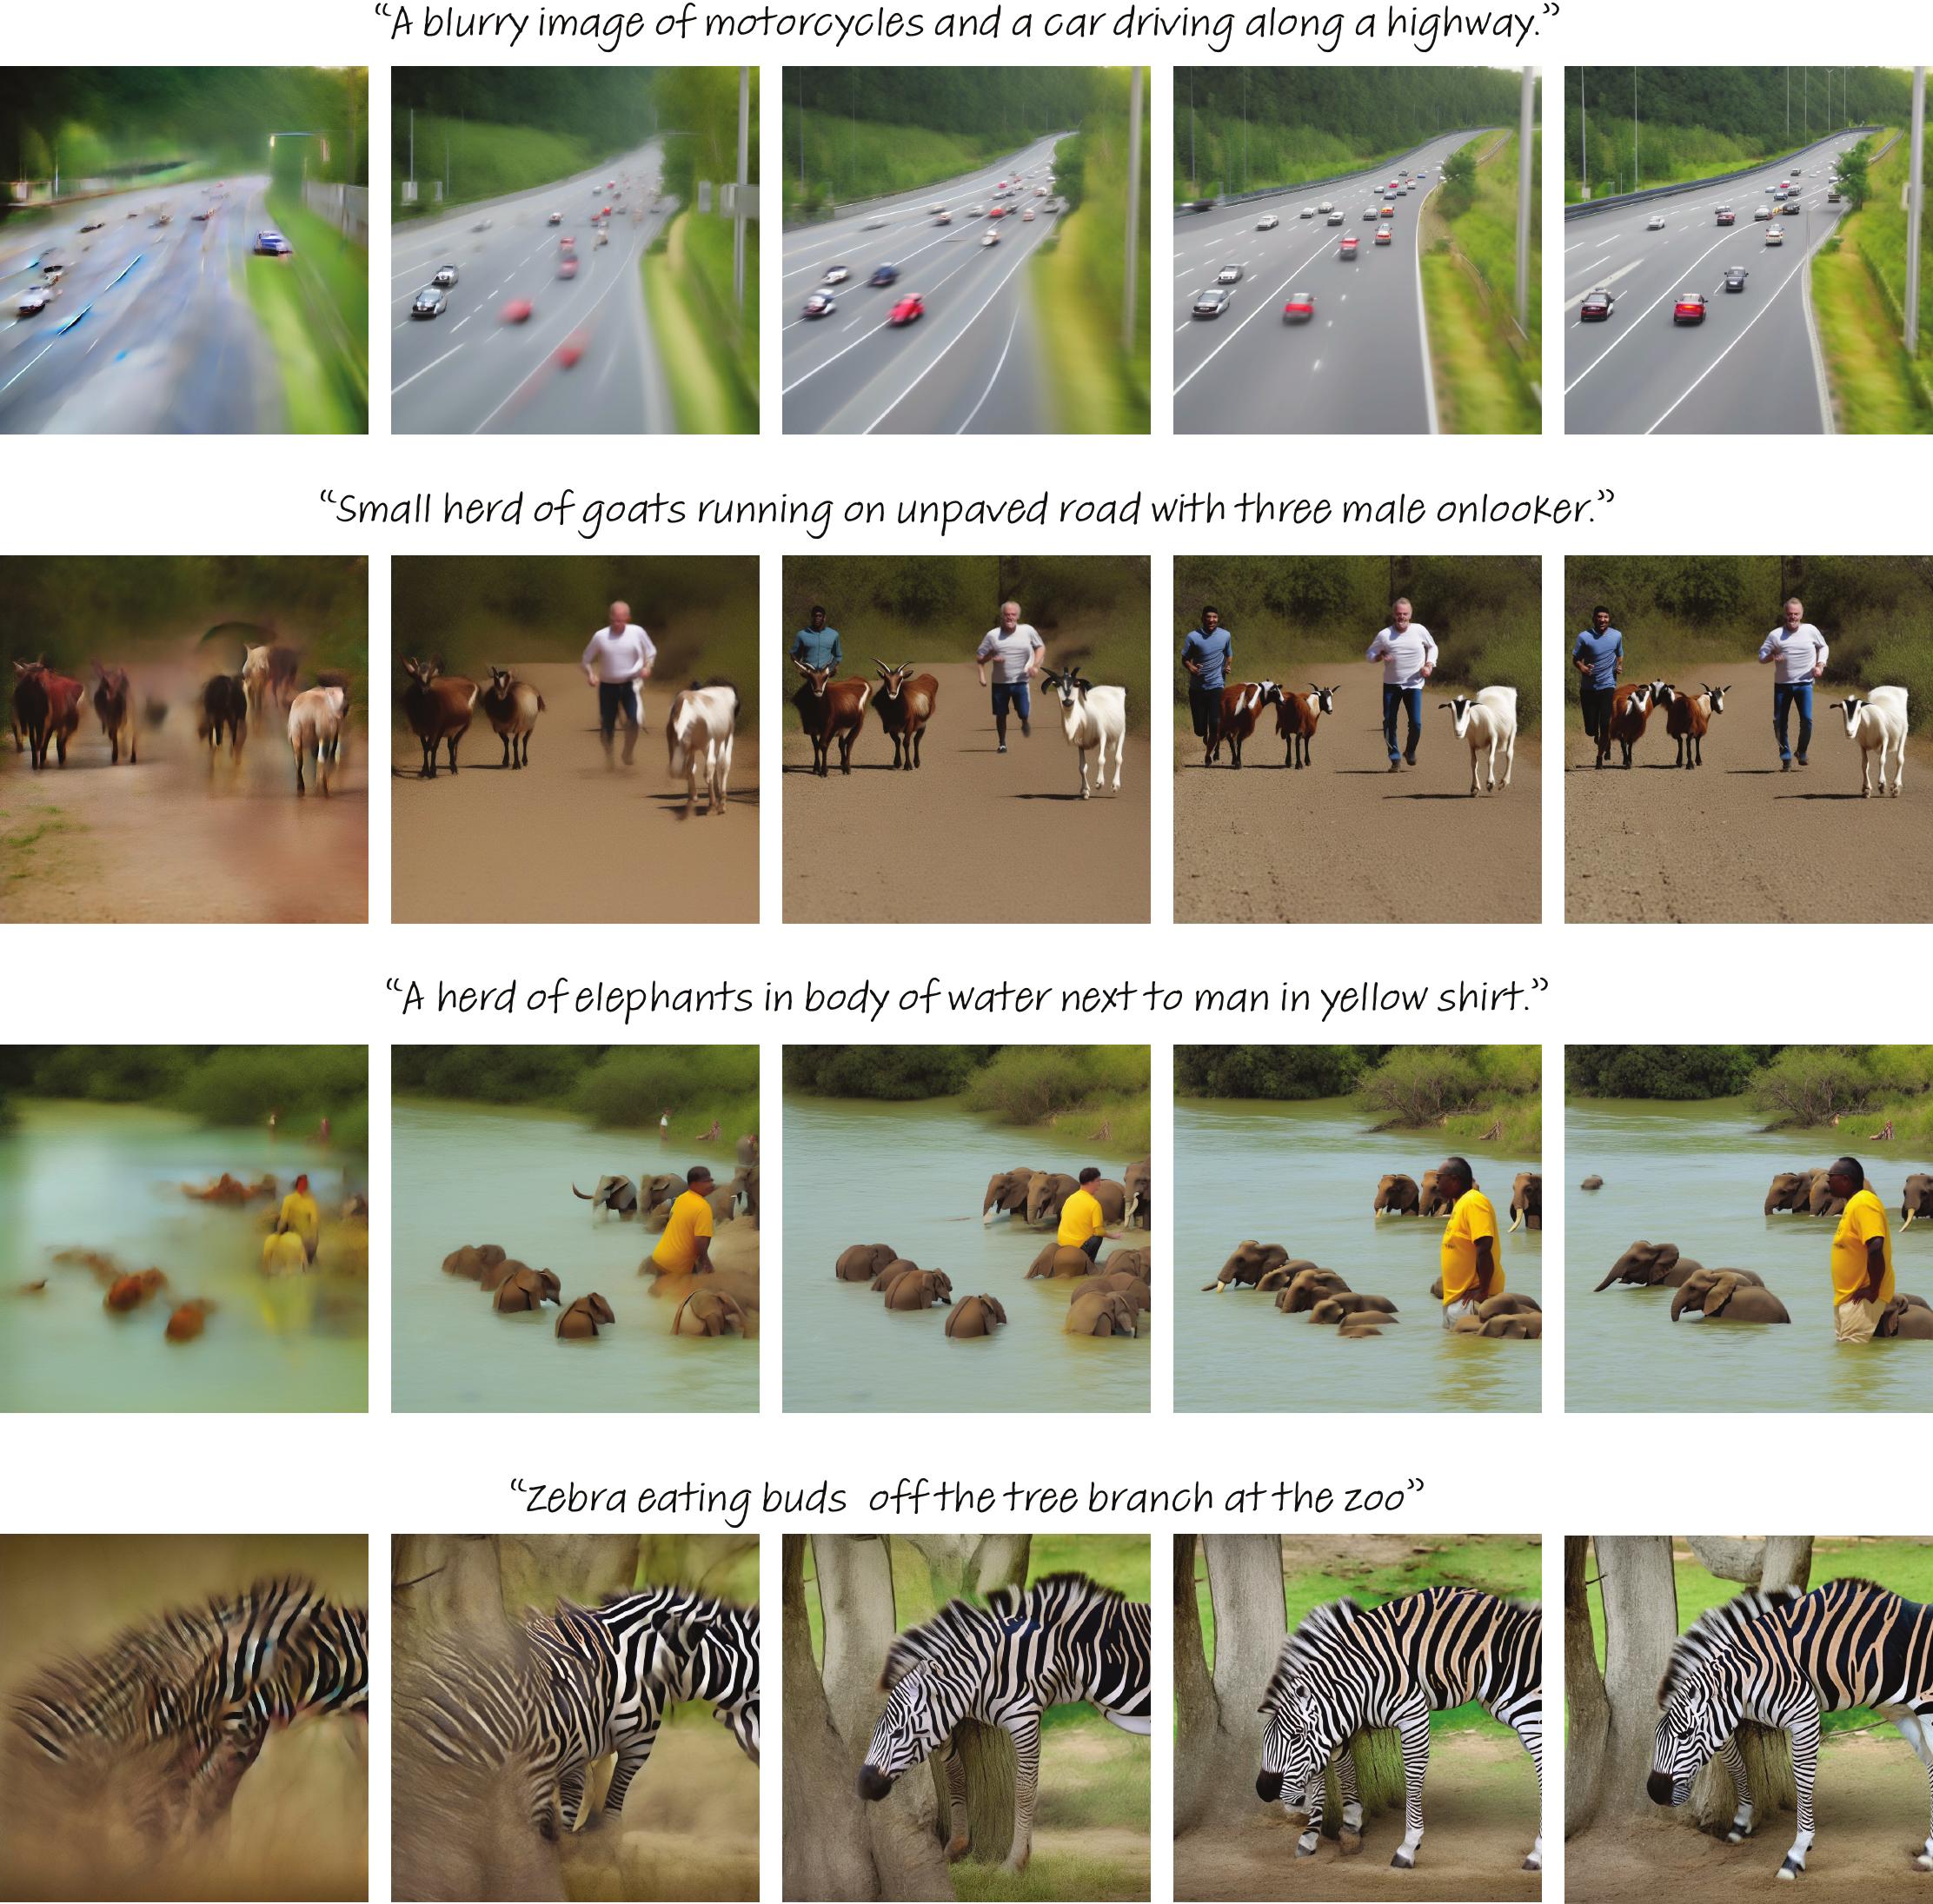}
  \Caption{
      Additional qualitative results at $t^*=9$.
  }{
    From left to right, the columns are $t=3,5,9,17,22$.
  }
  \label{fig:tileResults_9}
  \Description{}
\end{figure*}
